# Supplementary material for: Discovering and Mitigating Visual Biases through Keyword Explanation
Source: arXiv:2301.11104 source file (2024-03-27)
Supplement: Supplementary file 1 [file related.tex]

\section{Additional related works}
\label{appx:related}

\textbf{Bias and fairness.}
% fix by kyungmin
Biases in the datasets and models are a long-lasting problem in machine learning~\cite{torralba2011unbiased}. 
While there are broad studies on various types of biases~\cite{mehrabi2021survey}, we focus on the 
majority (specifically, group type and model-specific) biases. Namely, our goal is to investigate the failure of the classifier that the model fails for some subgroups (or attributes) of the dataset. This failure is highly related to the fairness issue, as the model often underperforms for specific gender~\cite{bolukbasi2016man,zhao2017men,hendricks2018women} or race~\cite{lee2018detecting,jalal2021fairness}. This failure is usually incurred by the imbalance in the dataset and further amplified during model training~\cite{johnson2019survey}. Imbalanced classification is highly related to the bias and fairness issue but developed independently following somewhat different setups~\cite{kim2020m2m,kim2020distribution}. We focus on the algorithmic solution for mitigating this bias or imbalance issue that strengthens the learning signal from minority samples~\cite{rahimian2019distributionally}, but balancing the samples in the data collection stage is a more important and effective step~\cite{roh2019survey}.

Not only the fairness issue (or improving the worst-group accuracy), the bias is also highly related to the generalization performance, particularly when in the presence of distribution shifts~\cite{muandet2013domain}. Indeed, the ratio of majority and minority samples can vary, which may make the model prone to changing their constitution. This is also related to the shortcut in learning that the model overly relies on spurious features instead of core features~\cite{geirhos2020shortcut}. There are various types of shortcuts, such as texture bias~\cite{geirhos2019imagenet}, background bias~\cite{xiao2021noise}, and scene bias~\cite{mo2021object}. We remark that our \sname framework could discover all these biases, e.g., ``illustration'' in ImageNet-R, ``forest'' and ``ocean'' in Waterbirds, and scene relation between ``toilet tissue'' and ``cat'' in ImageNet.

\textbf{Bias discovery.}
Discovering biases (or explaining failures) of models has been widely studied, especially under the domains where features are interpretable, such as table~\cite{zhang2018manifold,chung2019slice} or language~\cite{wu2019errudite,ribeiro2020beyond}. However, analyzing biases of visual models is more challenging since the features are hard to interpret for humans. To this end, some prior works aim to label the visual features by crowdsourcing~\cite{nushi2018towards,plumb2022finding,idrissi2022imagenet} or using a simulator~\cite{leclerc20213db}. These approaches provide human-readable information, but require heavy annotation costs and may not be feasible for some visual domains.

Another line of work leverages interpretable machine learning~\cite{molnar2020interpretable}, specifically visualization techniques such as feature visualization~\cite{olah2017feature,engstrom2019adversarial} or saliency map~\cite{selvaraju2017grad,adebayo2018sanity}. They assume the images are composed of core and spurious features and visualize the features (or mask the salient regions) for human interpretation~\cite{singla2021understanding,jain2022missingness}. However, these approaches are hard to interpret since they only provide sample-wise visualization, not summarized insights of entire datasets or models. Thus, succeeding research tries to provide higher-level insights by analyzing the features with decision tree~\cite{wong2021leveraging}, ranking~\cite{moayeri2022spuriosity}, and natural language description~\cite{hernandez2022natural}. Our work (\sname) is related to the final one called MILAN. However, MILAN aims to interpret the visual neurons, unlike \sname focuses on understanding mispredicted images. In addition, \sname provides bias keywords that the users can easily understand and use for various applications.

Some works aim to identify the biased samples from hard-to-learn (potentially biased) samples in a similar spirit of \sname. Precisely, they detect the biased samples by simply retrieving the mispredicted samples~\cite{liu2021just}, based on the training statistics~\cite{nam2020learning}, or clustering low-dimensional embeddings~\cite{sohoni2020no}. \sname better determines the biased samples by leveraging the pre-trained vision-language models. Furthermore, \sname defines various bias groups based on their language explanations, applicable to complex real-world datasets with multiple biases.

We propose an alternative direction for bias discovery: use vision-language (captioning) models. A few recent works use vision-language models to discover biases (they call slices or model failures). Concretely, they define biased groups as the outliers in the embedding space of the visual encoder, estimated by a Gaussian mixture model~\cite{eyuboglu2022domino} or support vector machine~\cite{jain2022distilling}. In contrast, we directly generate captions from images, which may contain more detailed information than the encoder embeddings. As a result, \sname can find multiple and fine-grained biases from descriptive captions. Recall that \sname only gives the suggestions of biases and the user makes the final decision, in contrast to the prior works finding the outliers first and then generating the description. It gives several advantages of \sname over prior works, e.g., \sname can effectively discover multiple potential biases without a repetitive finding of outliers.

Moreover, \sname has several technical and empirical contributions over the prior works. First, \sname can categorize the bias types as majority bias (e.g., ``hair'') or spurious correlation (e.g., ``man''), giving additional information for users. Using this information, we also train a debiased classifier by applying the group labels (for spurious correlation) inferred by \sname to GDRO~\cite{sagawa2020distributionally} algorithm; unlike prior works only consider resolving the model failures (without such group information) by intervention. Moreover, we demonstrate various applications of \sname, discovering novel biases from real-world datasets such as a gender bias ``player'' and ``shocked'' for the female class in Kaggle Face, and analyzing the differences between classifiers, e.g., ViT understands the global context better than ResNet.

\textbf{Debiasing classifiers.}
After identifying biases, a natural next step is to remove the biases from the classifiers. Numerous ideas were proposed under different names and assumptions, such as model debugging~\cite{singla2022data,shah2022modeldiff}, model editing~\cite{santurkar2021editing,mitchell2022fast}, and robust training~\cite{wang2019learning,arjovsky2019invariant}. They have different assumptions on biases (e.g., shortcuts like texture bias or minor groups for fairness) and training details (e.g., training from scratch or post-hoc fine-tuning for bias removal).

In this paper, we focus on distributionally robust optimization~\citep[DRO]{rahimian2019distributionally}, which aims to make the classifier robust to spurious correlations, i.e., improve the worst-group accuracy of minor groups. DRO is formulated as a minimax optimization $\min_f \max_a \ell(f,a)$ of minimizing the loss $\ell$ of the model $f$ maximized over the groups (or attributes) $a$. Many training algorithms for DRO were developed, including bi-level optimization~\cite{kim2019learning,sagawa2020distributionally,levy2020large,creager2021environment,zhang2022correct} or disentangling core and spurious features~\cite{lee2021learning}. However, DRO requires group (or bias) labels $a$ for every sample, demanding exhaustive annotation costs.

Thus, prior works attempted to reduce the labeling cost by estimating the bias labels in an unsupervised~\cite{bahng2020learning,nam2020learning,sohoni2020no,liu2021just,bao2022learning} manner.\footnote{
Some works also consider semi-supervised~\cite{sohoni2021barack,nam2022spread} setups.
} 
However, the unsupervised bias discovery methods are often inaccurate and not expandable for multiple biases, e.g., cannot distinguish ``shocked'' and ``player'' for gender classification. In contrast, \sname accurately infers the labels of multiple biases in a ``zero-shot'' manner, leveraging the power of vision-language models. 
Similar to the success of zero-shot image classification~\cite{radford2021learning}, we claim that the discovery of bias and sample-wise labeling should also be done in a zero-shot manner.

% fix by kyungmin
We remark that bias labeling in a zero-shot manner is not trivial. \citet{zhang2022contrastive} attempted to use CLIP for estimating the sample-wise bias labels (given that the ``bias keyword'' is known), but directly using group names might lead to inferior performance, e.g., see Table~\ref{tab:f1score} for Waterbirds dataset.  In contrast, \sname predicts the bias labels reasonably well, and using them for prompt tuning significantly improves the zero-shot classification without fine-tuning. Moreover, \sname finds the potential unknown biases, which can be more challenging than annotating sample-wise labels of the known bias.

\textbf{Vision-language models.}
Vision-language models have shown remarkable success by pre-training from large-scale image-text pairs~\cite{bommasani2021opportunities}. 
They can be categorized into: joint embedding of image and text modalities~\cite{radford2021learning,lu2019vilbert}, image-to-text~\cite{desai2021virtex,li2022blip}, text-to-image~\cite{ramesh2021zero}, and hybrid~\cite{wang2022unifying} models. Our \sname framework can be applied to any type of model that can generate captions (i.e., image-to-text) to predict the bias keywords, although we need a joint embedding model to determine the bias types further. 
Therefore, in our main experiments, we choose CLIP~\cite{radford2021learning} as the default joint embedding model and ClipCap~\cite{mokady2021clipcap} which is built upon CLIP embeddings, as the default image captioning model. 
For completeness, we also test other image captioning models such as BLIP~\cite{li2022blip} and OFA~\cite{wang2022unifying} in Appendix~\ref{appx:comp_caption}, and confirm that different image captioning models give reasonably consistent results.
