# Supplementary material for: Discovering and Mitigating Visual Biases through Keyword Explanation
Source: arXiv:2301.11104 source file (2024-03-27)
Supplement: Supplementary file 2 [file comp_dro.tex]

\begin{table*}[ht!]
\caption{
Comparison of ERM vs. GDRO.
}\label{tab:comp-dro}
\vspace{-0.05in}
% \vspace{-0.08in}
% \newcommand{\gap}[1]{{\color{red}#1}}
%
\begin{subtable}{0.33\textwidth}
\centering\small
\captionsetup{justification=centering}
\caption{CelebA blond}
% \vspace{-0.04in}
\resizebox{\textwidth}{!}{% 
\begin{tabular}{lccc}
\toprule
\phantom{biological species}
& ERM & GDRO & Gap \\
% \midrule
% \rowcolor{lightgray}
% worst-group acc. & \phantom{-}39.6 & \phantom{-}91.8 & \phantom{-}54.9 \\ 
\midrule
man                 & \phantom{-}1.22 & \xmark & \gap{\xmark} \\ 
player              & \phantom{-}0.42 & \xmark & \gap{\xmark} \\
person              & \phantom{-}0.17 & \phantom{-}0.05 & -0.12 \\ 
artist              & \phantom{-}0.16 & \xmark & \xmark \\ 
comedy              & \phantom{-}0.16 & \xmark & \xmark \\
film                & \phantom{-}0.13 & \phantom{-}0.48 & +0.32 \\  
actor               & \phantom{-}0.08 & -0.38 & -0.40 \\ 
face                & \phantom{-}0.06 & \xmark & \xmark \\
love                & \phantom{-}0.06 & \phantom{-}0.36 & +0.30 \\ 
clothing            & \phantom{-}0.05 & \phantom{-}0.16 & +0.11 \\ 
\bottomrule
\end{tabular}}
\end{subtable}
\begin{subtable}{0.33\textwidth}
\centering\small
\caption{Waterbird}
% \vspace{-0.04in}
\resizebox{\textwidth}{!}{% 
\begin{tabular}{lccc}
\toprule
\phantom{biological species}
& ERM & GDRO & Gap \\
% \midrule
% \rowcolor{lightgray}
% worst-group acc. & \phantom{-}57.1 & \phantom{-}77.4 & \phantom{-}20.3 \\ 
\midrule
forest              & \phantom{-}2.12 & \phantom{-}1.83 & \gap{-0.29} \\ 
woods               & \phantom{-}1.94 & \phantom{-}1.67 & \gap{-0.27} \\ 
tree                & \phantom{-}1.45 & \phantom{-}1.66 & \gap{+0.21} \\ 
branch              & \phantom{-}1.20 & \phantom{-}1.23 & \gap{+0.03} \\ 
prey                & \phantom{-}0.20 & \xmark & \xmark \\
wild                & \phantom{-}0.19 & \xmark & \xmark \\
bird of prey        & -0.03 & \xmark & \xmark \\
species             & -0.05 & \phantom{-}0.03 & +0.08 \\ 
area                & -0.09 & \phantom{-}0.13 & +0.24 \\ 
biological species  & -0.11 & \phantom{-}0.08 & +0.19 \\ 
\bottomrule
\end{tabular}}
\end{subtable}
\begin{subtable}{0.33\textwidth}
\centering\small
\caption{Landbird}
% \vspace{-0.04in}
\resizebox{\textwidth}{!}{% 
\begin{tabular}{lccc}
\toprule
\phantom{biological species}
& ERM & GDRO & Gap \\
% \midrule
% \rowcolor{lightgray}
% worst-group acc. & \phantom{-}80.0 & \phantom{-}87.6 & \phantom{-}7.6 \\ 
\midrule
ocean               & \phantom{-}3.41 & 1.98 & \gap{-1.43} \\
beach               & \phantom{-}2.83 & 1.39 & \gap{-1.45} \\
surfer              & \phantom{-}2.73 & 1.55 & \gap{-1.18} \\
boat                & \phantom{-}2.16 & 1.14 & \gap{-1.02} \\
dock                & \phantom{-}1.56 & 0.59 & \gap{-0.97} \\
water               & \phantom{-}1.38 & 0.84 & \gap{-0.54} \\
lake                & \phantom{-}1.17 & \xmark & \gap{\xmark} \\
rocks               & \phantom{-}1.02 & \xmark & \gap{\xmark} \\
sunset              & \phantom{-}0.88 & \xmark & \gap{\xmark} \\
kite                & \phantom{-}0.67 & \xmark & \gap{\xmark} \\
\bottomrule
\end{tabular}}
\end{subtable}
\vspace{-0.05in}
\end{table*}
